# Supplementary material for: Quantum (in)stability of maximally symmetric space-times
Source: arXiv:2303.11091 ancillary file (2023-12-08)
Supplement: Supplementary file 1 [file animated_gifs.pdf]

# Supplementary material

## 1 Animated gifs

Five animated gifs are given as ancillary files. They show the poles of the spin-2 propagator for different choices of parameters. These two parameters are the background curvature in units of the species scale $GN^2\bar{R}$ and the coefficient $\tilde{\alpha}$ multiplying the $R^2$ term of the gravitational action.

The animation time corresponds to different values of $\tilde{\beta}_{\text{eff}}$, going from large and negative values to large and positive values. Each colored dot corresponds to a pole located in the complex plane for $\nu$ (or $k$ for flat space). A green dot indicates a non-ghostly pole, whereas a red dot is a ghost and a purple dot is a pole with complex residue.

With these two parameters fixed, the position of the poles only depends on $a$ defined by

$$a \equiv \frac{GN^2\bar{R}}{6}\left[2\left(\frac{12\pi}{GN^2\bar{R}} - \tilde{\alpha}\right) - 1\right]\exp\left\{\tilde{\beta}_{\text{eff}} - \frac{1}{2} + 2\gamma_E\right\}. \tag{1.1}$$

In flat space, this quantity is given by

$$a \underset{\bar{R}=0}{=} 4\pi e^{\tilde{\beta}_{\text{eff}} - \frac{1}{2} + 2\gamma_E} \tag{1.2}$$

The animated gifs are listed below:

- The file "flat.gif" corresponds to flat (Minkowski) spacetime $GN^2\bar{R} = 0$, for which the spin-2 perturbations are independent of $\tilde{\alpha}$
- The file "dS_alpha0_H4pi.gif" corresponds to de Sitter spacetime with $GN^2H^2 = 4\pi$ and $\tilde{\alpha} = 0$. As a consequence, the quantity $a$ defined in (1.1) is always negative and we observe that the two tachyons stay on the real axis after they have merged.

- The file “dS_alpha-1_H2pi.gif” corresponds to de Sitter spacetime with $GN^2H^2 = 2\pi$ and $\tilde{\alpha} = -2$. As a consequence, $a$ (1.1) is always positive and we observe that the two tachyons become a pair of complex conjugates after they have merged on the real axis.

- The file “AdS_alpha0_chi2pi.gif” corresponds to anti-de Sitter spacetime with $GN^2\chi^2 = 2\pi$ and $\tilde{\alpha} = 0$. As a consequence, $a$ (1.1) is always positive and we observe that the two tachyons become a pair of complex conjugates after they have merged on the imaginary axis.

- The file “AdS_alpha-2_chi2pi.gif” corresponds to anti-de Sitter spacetime with $GN^2\chi^2 = 2\pi$ and $\tilde{\alpha} = -2$. As a consequence, $a$ (1.1) is always negative and we observe that the two tachyons stay on the imaginary axis after they have merged.
